# Supplementary material for: HandFlow: Quantifying View-Dependent 3D Ambiguity in Two-Hand Reconstruction with Normalizing Flow
Source: arXiv:2210.01692 source file (2022-10-04)
Supplement: Supplementary file 1 [file AblationFigure.tex]

\begin{figure}[hbt!]
  \includegraphics[width=0.24\linewidth]{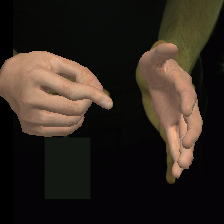}
  \includegraphics[width=0.24\linewidth]{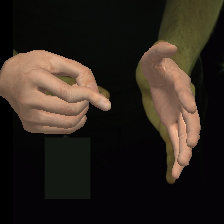}
  \includegraphics[width=0.24\linewidth]{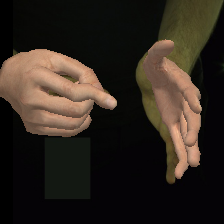}
  \includegraphics[width=0.24\linewidth]{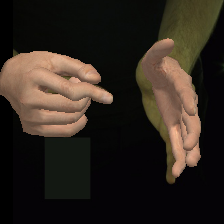}
  \includegraphics[width=0.24\linewidth]{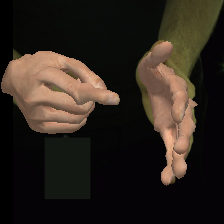}
  \includegraphics[width=0.24\linewidth]{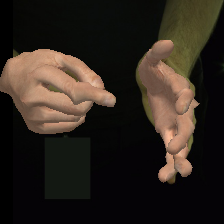}
  \includegraphics[width=0.24\linewidth]{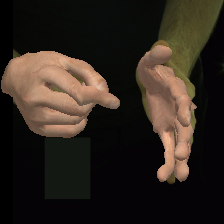}
  \includegraphics[width=0.24\linewidth]{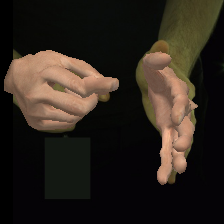}
  
  \includegraphics[width=0.24\linewidth]{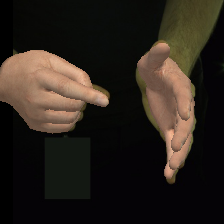}
  \includegraphics[width=0.24\linewidth]{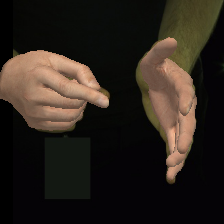}
  \includegraphics[width=0.24\linewidth]{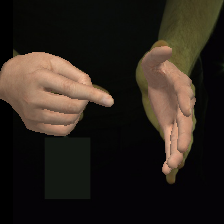}
  \includegraphics[width=0.24\linewidth]{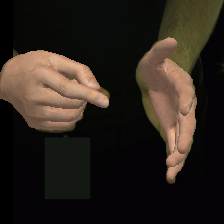}

  \caption{w/o $\mathcal{L}_{\text{Param}}$ (Top) and or w/o $\mathcal{L}_{\text{RotReg}}$ (Middle), ambiguity in joint supervision leads to unnatural twist rotations in samples. These ambiguities are reduced for our full method (Bottom).}
  \label{fig:ablation}
\end{figure}
