# Supplementary material for: HandFlow: Quantifying View-Dependent 3D Ambiguity in Two-Hand Reconstruction with Normalizing Flow
Source: arXiv:2210.01692 source file (2022-10-04)
Supplement: Supplementary file 2 [file FuzzyResults_new.tex]

{
\newcommand{\ImageWidthSupp}{0.16}
\newcommand{\ImageHSepSupp}{0.1cm}
\newcommand{\ImageVSepSupp}{0.1cm}
\newcommand{\TitleVSepSupp}{0.35cm}
\begin{figure*}
  \centering
  \begin{tikzpicture}[every node/.style={inner sep=0,outer sep=0}]%
  % first row
  \node (image_IH_1_input) at (0,0) {\includegraphics[trim=0 1.2cm 0 1.2cm, clip, width=\ImageWidthSupp\linewidth]{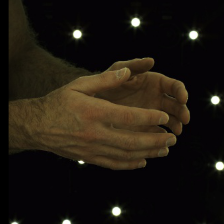}};
  \node[above=\TitleVSepSupp of image_IH_1_input, anchor=north] {\small{Input}};
  \node[right=\ImageHSepSupp of image_IH_1_input, anchor=west] (image_IH_1_cam)  {\includegraphics[trim=2cm 1cm 2cm 1cm, clip, width=\ImageWidthSupp\linewidth]{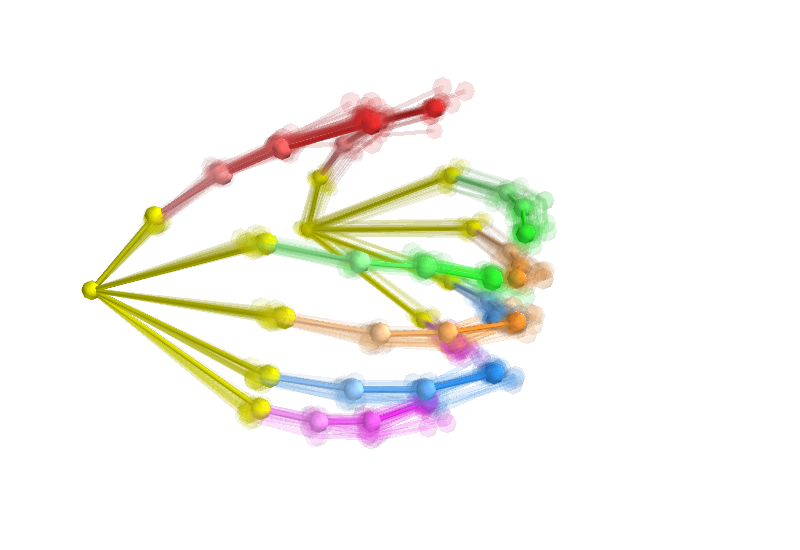}};
  \node[above=\TitleVSepSupp of image_IH_1_cam, anchor=north] {\small{Camera View}};
  \node[right=\ImageHSepSupp of image_IH_1_cam, anchor=west] (image_IH_1_side) {\includegraphics[trim=2cm 1cm 2cm 1cm, clip, width=\ImageWidthSupp\linewidth]{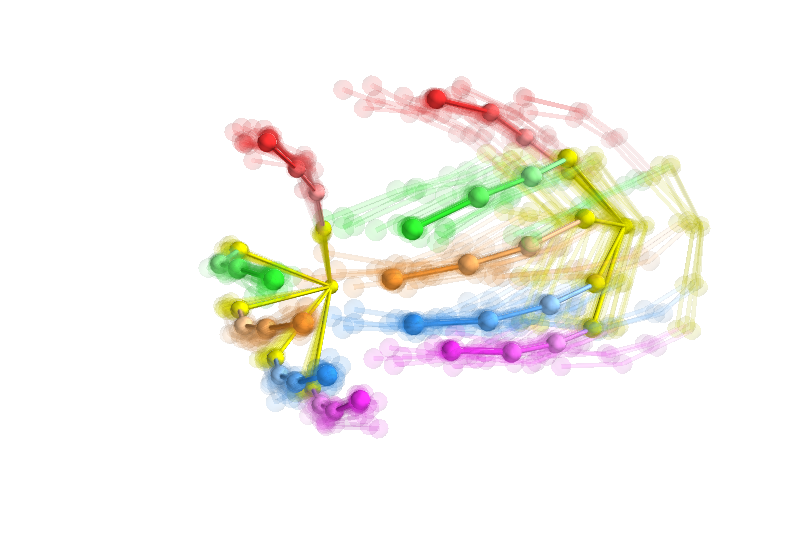}};
  \node[above=\TitleVSepSupp of image_IH_1_side, anchor=north] {\small{Side View}};
  \node[right=\ImageHSepSupp of image_IH_1_side] (image_Tz_1_input) {\includegraphics[trim=0 1.2cm 0 1.2cm, clip, width=\ImageWidthSupp\linewidth]{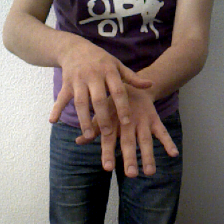}};
  \node[above=\TitleVSepSupp of image_Tz_1_input, anchor=north] {\small{Input}};
  \node[right=\ImageHSepSupp of image_Tz_1_input] (image_Tz_1_cam) {\includegraphics[width=\ImageWidthSupp\linewidth]{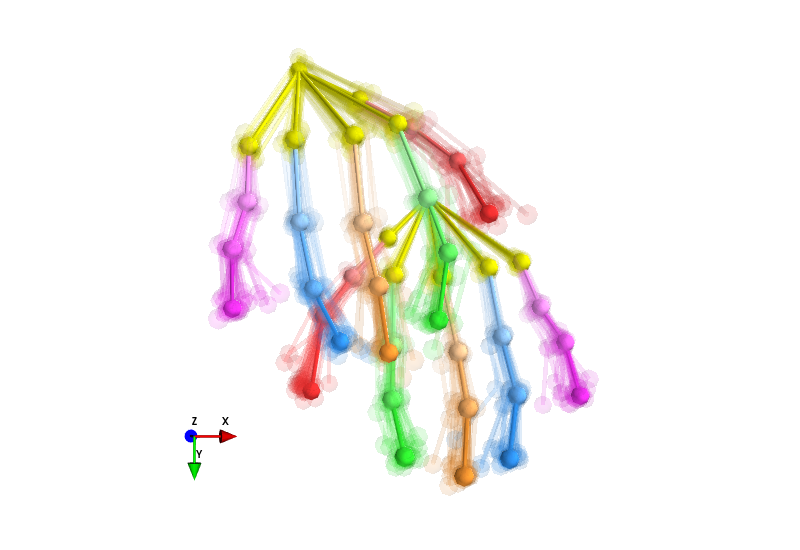}};
  \node[above=\TitleVSepSupp of image_Tz_1_cam, anchor=north] {\small{Camera View}};
  \node[right=\ImageHSepSupp of image_Tz_1_cam] (image_Tz_1_side) {\includegraphics[width=\ImageWidthSupp\linewidth]{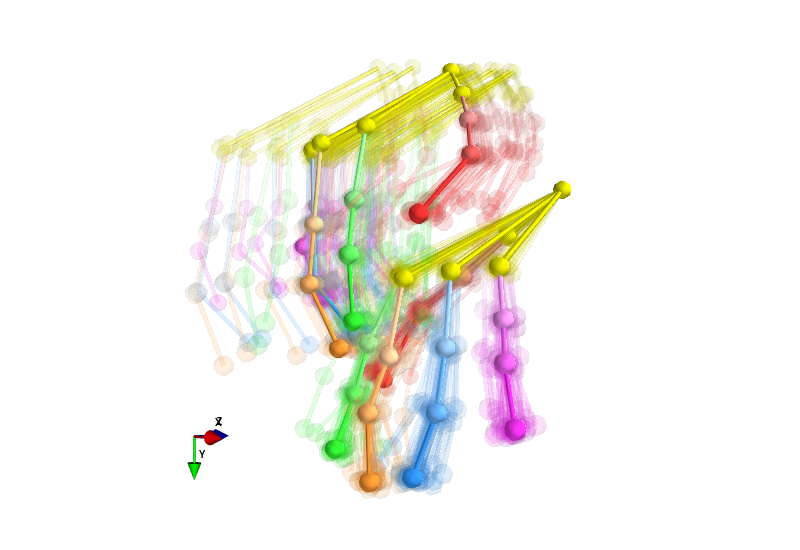}};
  \node[above=\TitleVSepSupp of image_Tz_1_side, anchor=north] {\small{Side View}};
  %
  % second row
  \node[below=\ImageVSepSupp of image_IH_1_input, anchor=north] (image_IH_2_input) {\includegraphics[trim=0 1.2cm 0 1.2cm, clip, width=\ImageWidthSupp\linewidth]{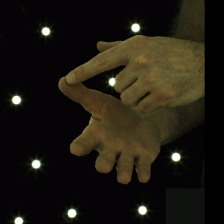}};
  \node[right=\ImageHSepSupp of image_IH_2_input, anchor=west] (image_IH_2_cam) {\includegraphics[trim=2cm 2cm 2cm 1cm, clip, width=\ImageWidthSupp\linewidth]{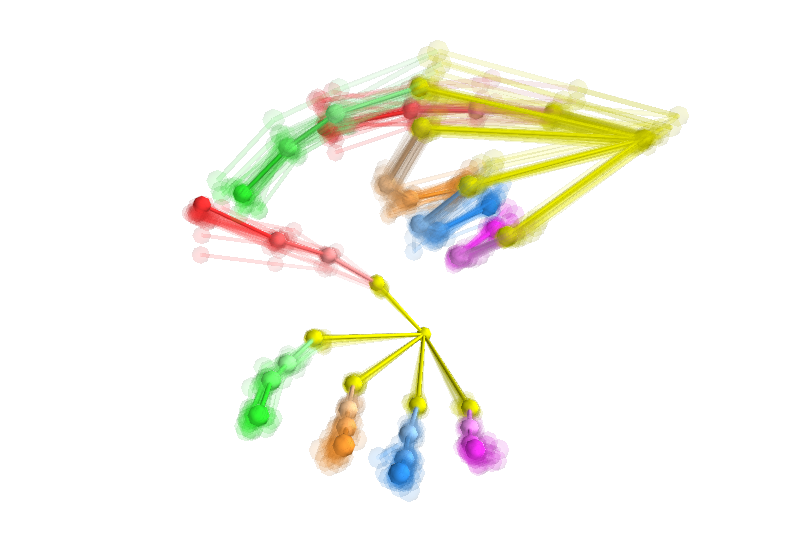}};
  \node[right=\ImageHSepSupp of image_IH_2_cam, anchor=west] (image_IH_2_side) {\includegraphics[width=\ImageWidthSupp\linewidth]{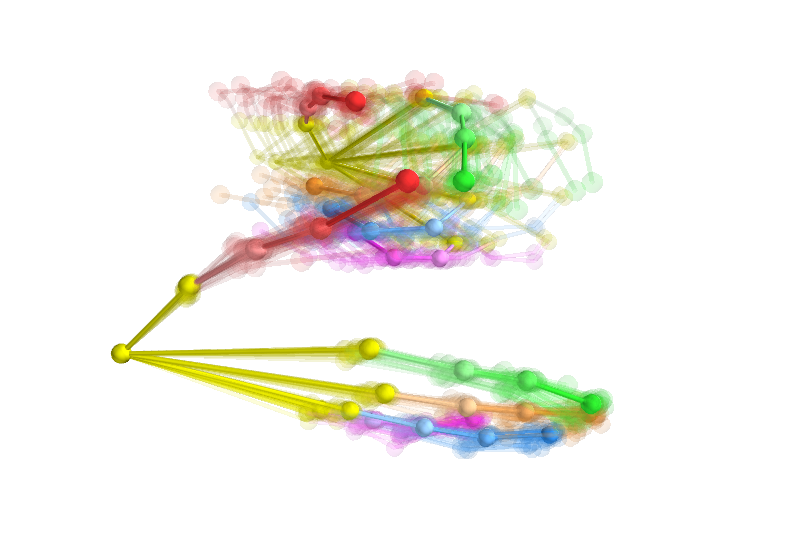}};
  \node[right=\ImageHSepSupp of image_IH_2_side, anchor=west] (image_Tz_2_input) {\includegraphics[trim=0 1.2cm 0 1.2cm, clip, width=\ImageWidthSupp\linewidth]{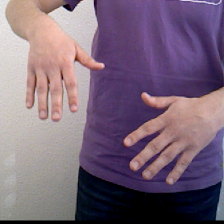}};
  \node[right=\ImageHSepSupp of image_Tz_2_input, anchor=west] (image_Tz_2_cam) {\includegraphics[width=\ImageWidthSupp\linewidth]{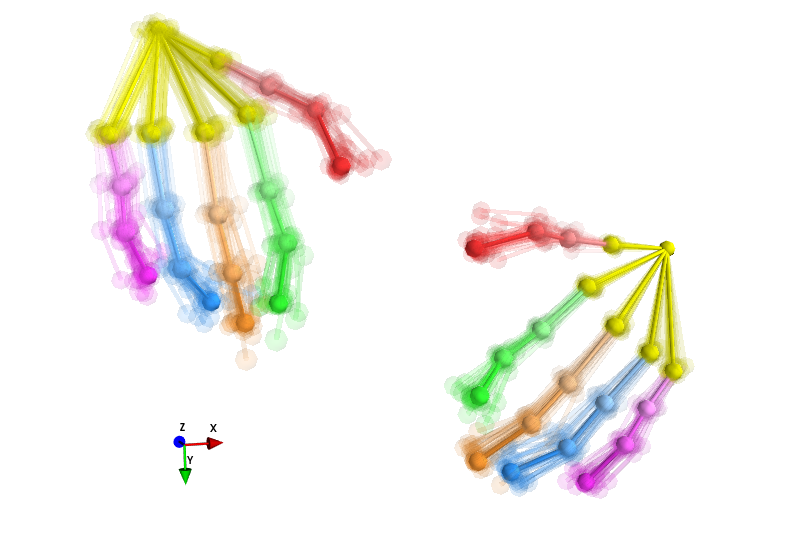}};
  \node[right=\ImageHSepSupp of image_Tz_2_cam, anchor=west] (image_Tz_2_side) {\includegraphics[width=\ImageWidthSupp\linewidth]{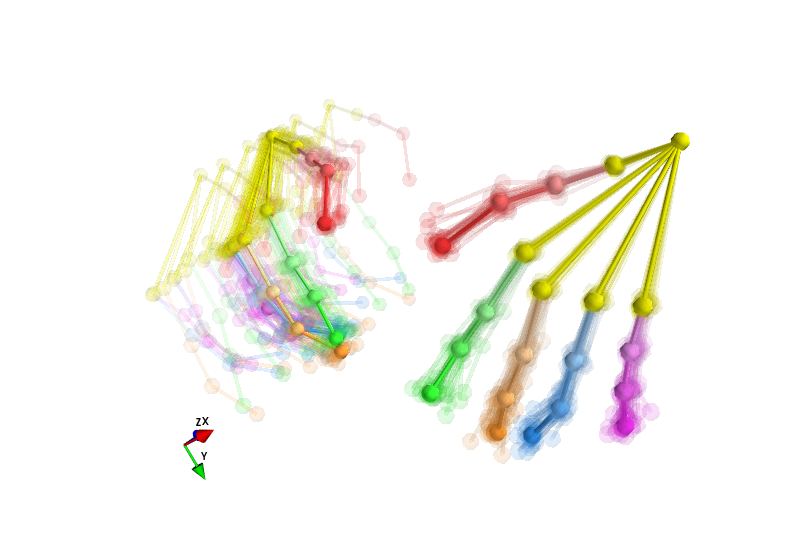}};
  %
  % third row
  \node[below=\ImageVSepSupp of image_IH_2_input, anchor=north] (image_IH_3_input) {\includegraphics[trim=0 1.2cm 0 1.2cm, clip, width=\ImageWidthSupp\linewidth]{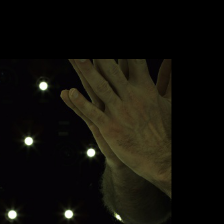}};
  \node[right=\ImageHSepSupp of image_IH_3_input, anchor=west] (image_IH_3_cam) {\includegraphics[trim=2cm 2cm 2cm 1cm, clip, width=\ImageWidthSupp\linewidth]{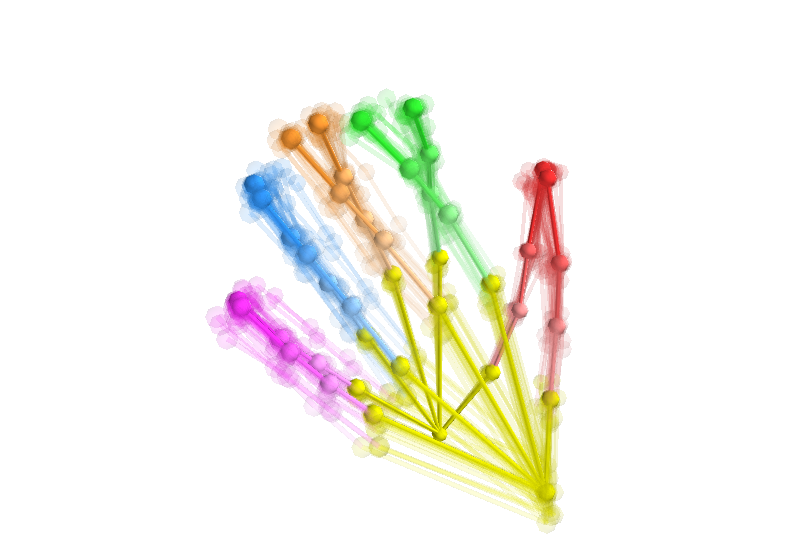}};
  \node[right=\ImageHSepSupp of image_IH_3_cam, anchor=west] (image_IH_3_side) {\includegraphics[trim=2cm 2cm 2cm 1cm, clip, width=\ImageWidthSupp\linewidth]{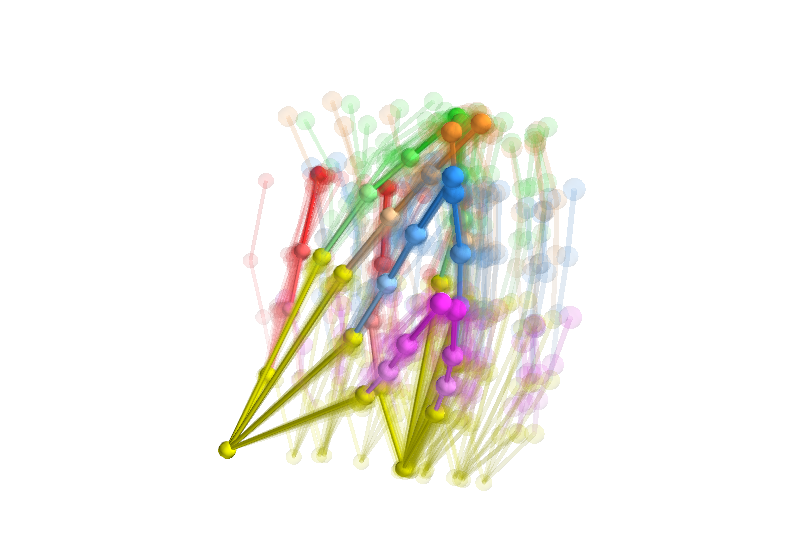}};
  \node[right=\ImageHSepSupp of image_IH_3_side, anchor=west] (image_Tz_3_input) {\includegraphics[trim=0 1.2cm 0 1.2cm, clip, width=\ImageWidthSupp\linewidth]{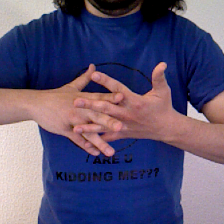}};
  \node[right=\ImageHSepSupp of image_Tz_3_input, anchor=west] (image_Tz_3_cam) {\includegraphics[width=\ImageWidthSupp\linewidth]{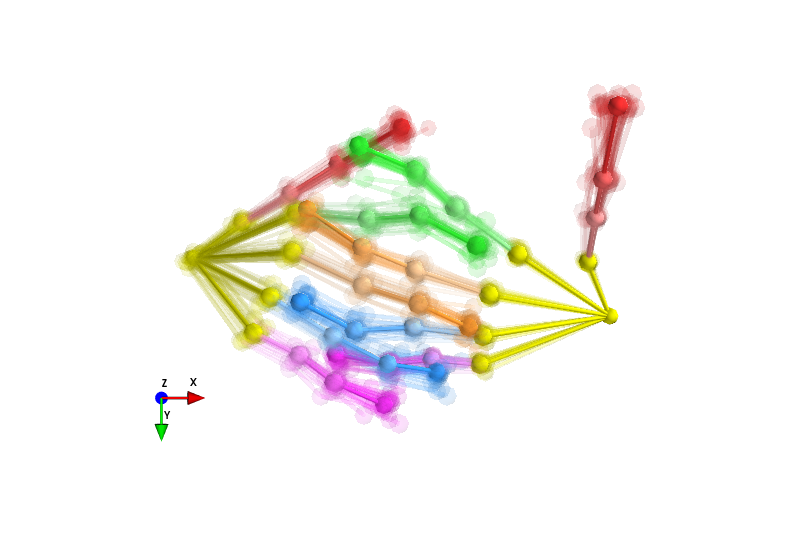}};
  \node[right=\ImageHSepSupp of image_Tz_3_cam, anchor=west] (image_Tz_3_side) {\includegraphics[width=\ImageWidthSupp\linewidth]{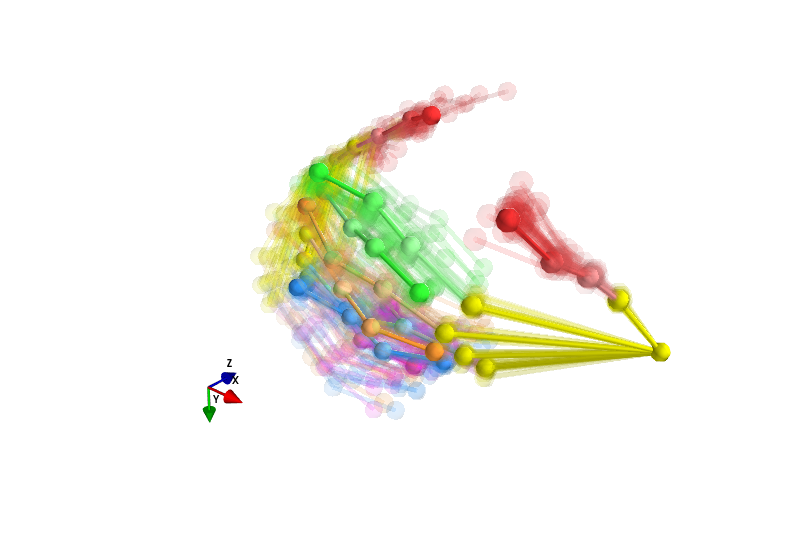}};
  %
  % fourth row
  \node[below=\ImageVSepSupp of image_IH_3_input, anchor=north] (image_IH_4_input) {\includegraphics[trim=0 1.2cm 0 1.2cm, clip, width=\ImageWidthSupp\linewidth]{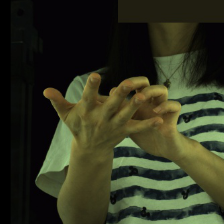}};
  \node[right=\ImageHSepSupp of image_IH_4_input, anchor=west] (image_IH_4_cam) {\includegraphics[trim=2cm 2cm 2cm 1cm, clip, width=\ImageWidthSupp\linewidth]{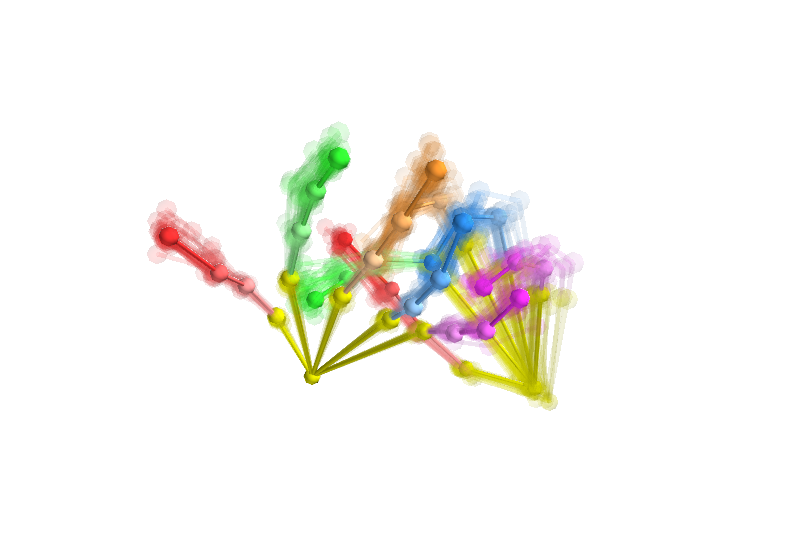}};
  \node[right=\ImageHSepSupp of image_IH_4_cam, anchor=west] (image_IH_4_side) {\includegraphics[trim=2cm 2cm 2cm 1cm, clip, width=\ImageWidthSupp\linewidth]{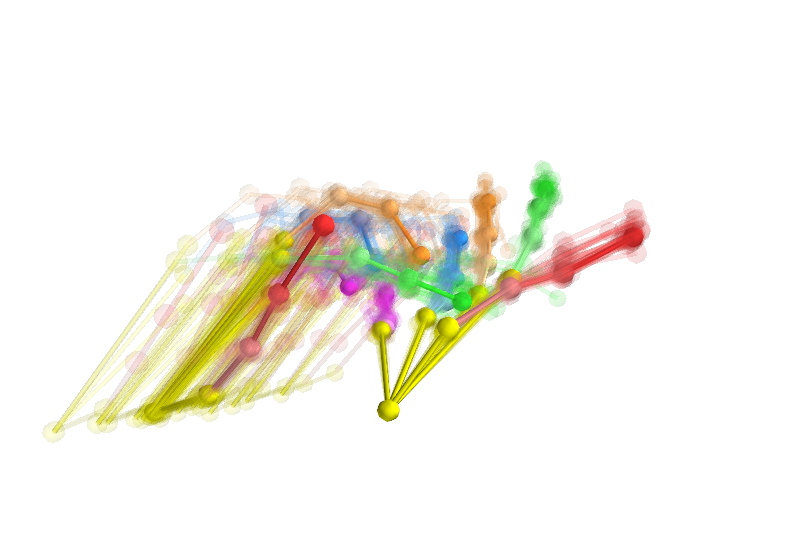}};
  \node[right=\ImageHSepSupp of image_IH_4_side, anchor=west] (image_Tz_4_input) {\includegraphics[trim=0 1.2cm 0 1.2cm, clip, width=\ImageWidthSupp\linewidth]{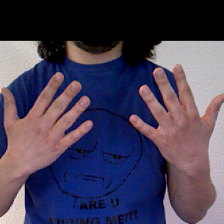}};
  \node[right=\ImageHSepSupp of image_Tz_4_input, anchor=west] (image_Tz_4_cam) {\includegraphics[width=\ImageWidthSupp\linewidth]{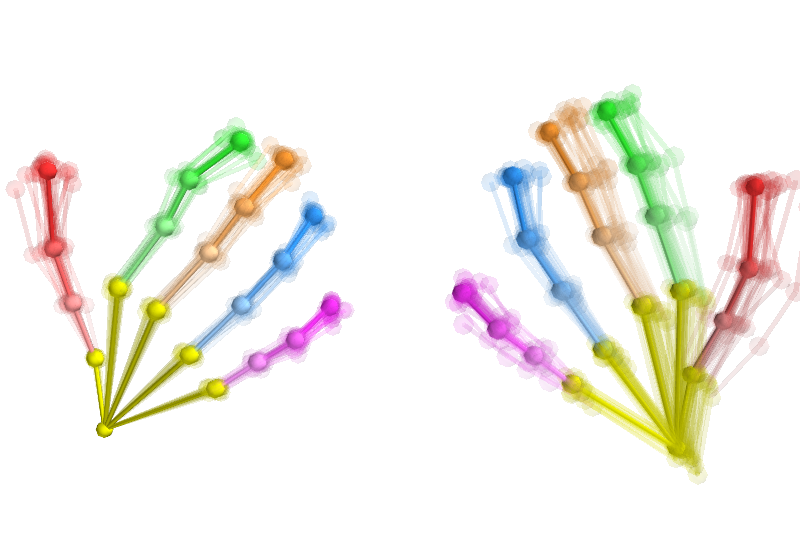}};
  \node[right=\ImageHSepSupp of image_Tz_4_cam, anchor=west] (image_Tz_4_side) {\includegraphics[width=\ImageWidthSupp\linewidth]{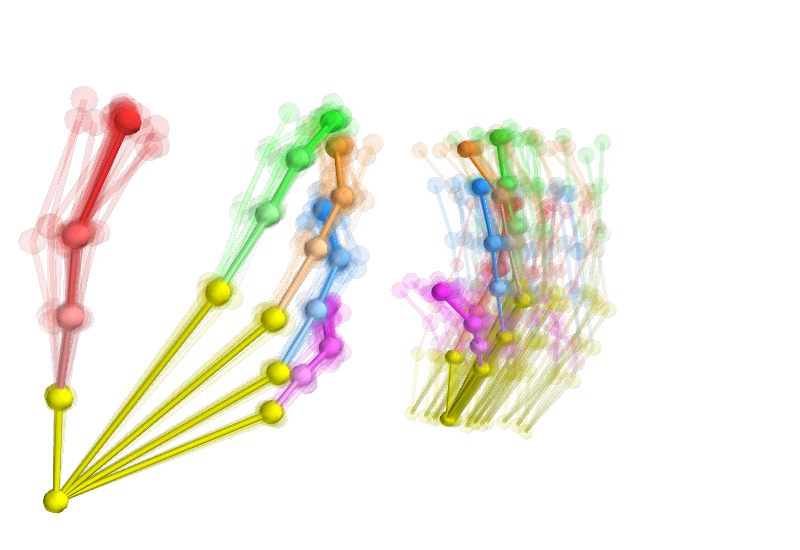}};
  \end{tikzpicture}
  \caption{
    We show 30 samples from the estimated distribution, rendered as semi-transparent skeletons, superimposed on a single image. These Samples are aligned to the root joint of one hand and the mode of the distribution is made opaque for ease of visualization. 
    Here we show more results from both the InterHand2.6M~\cite{moon2020interhand2} and the Tzionas~\cite{tzionas_ijcv2016} datasets.
  }
  \label{fig:FuzzySupp}
\end{figure*}
}
