# Supplementary material for: HandFlow: Quantifying View-Dependent 3D Ambiguity in Two-Hand Reconstruction with Normalizing Flow
Source: arXiv:2210.01692 source file (2022-10-04)
Supplement: Supplementary file 3 [file GroundTruthVis.tex]

\newcommand{\ImageWidthGT}{0.118}
\newcommand{\ImageHSepGT}{0.05cm}
\newcommand{\ImageHSepGTH}{0.025cm}
\newcommand{\ImageVSepGT}{0.05cm}
\newcommand{\ImageBlockHSepGT}{0.2cm}
\newcommand{\ImageBlockVSepGT}{0.2cm}
\newcommand{\TitleHSepGT}{0.15cm}
\newcommand{\TitleVSepGT}{0.35cm}
\newcommand{\BoxThicknessGT}{semithick}
\begin{figure*}
  \centering
  \begin{tikzpicture}[every node/.style={inner sep=0,outer sep=0}]%
  % first row, left side
  \node (image_GT_1) at (0,0) {\includegraphics[trim={0 4cm 0 4cm},clip, width=\ImageWidthGT\linewidth]{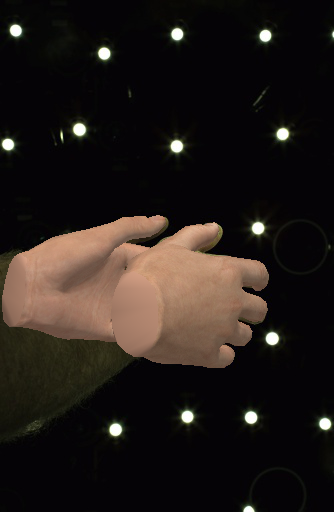}};
  \node[right=\ImageHSepGT of image_GT_1, anchor=west] (image_S_1_1) {\includegraphics[trim={0 4cm 0 4cm},clip, width=\ImageWidthGT\linewidth]{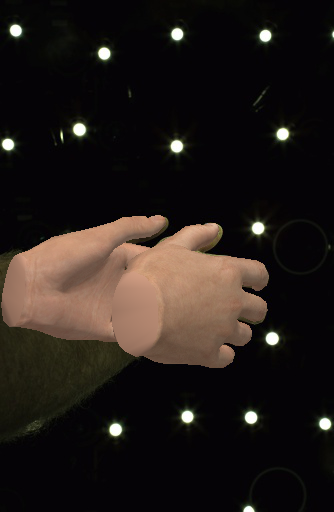}};
  \node[right=\ImageHSepGT of image_S_1_1, anchor=west] (image_S_1_2) {\includegraphics[trim={0 4cm 0 4cm},clip, width=\ImageWidthGT\linewidth]{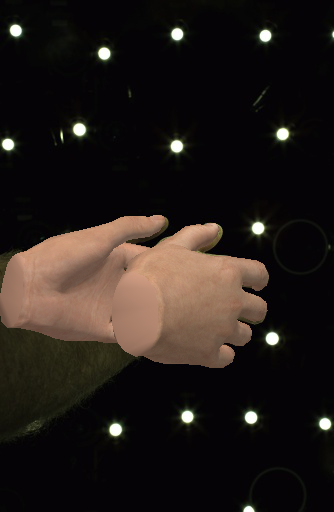}};
  \node[right=\ImageHSepGT of image_S_1_2, anchor=west] (image_S_1_3)
  {\includegraphics[trim={0 4cm 0 4cm},clip, width=\ImageWidthGT\linewidth]{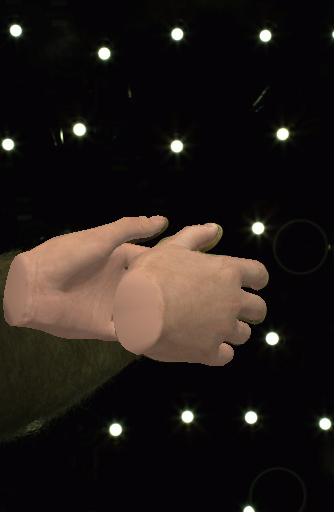}};
  %
  % first row, right side
  \node[right=\ImageBlockHSepGT of image_S_1_3, anchor=west] (image_GT_2) {\includegraphics[trim={0 2cm 0 6cm},clip,width=\ImageWidthGT\linewidth]{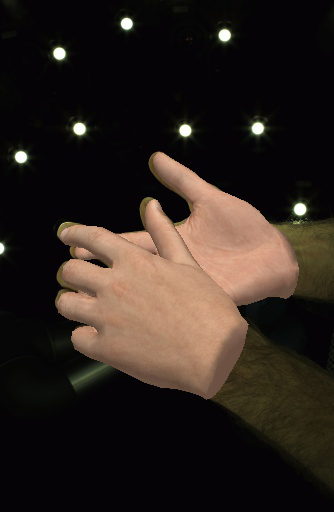}};
  \node[right=\ImageHSepGT of image_GT_2, anchor=west] (image_S_2_1) {\includegraphics[trim={0 2cm 0 6cm},clip,width=\ImageWidthGT\linewidth]{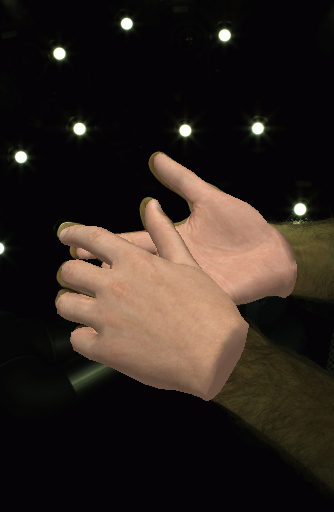}};
  \node[right=\ImageHSepGT of image_S_2_1, anchor=west] (image_S_2_2) {\includegraphics[trim={0 2cm 0 6cm},clip,width=\ImageWidthGT\linewidth]{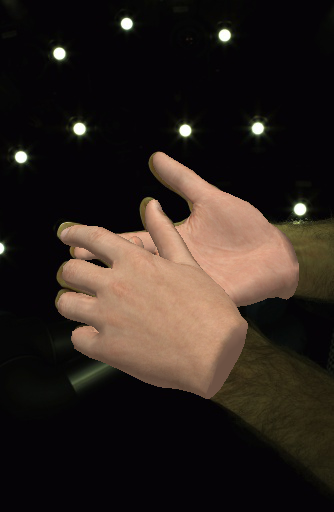}};
  \node[right=\ImageHSepGT of image_S_2_2, anchor=west] (image_S_2_3) {\includegraphics[trim={0 2cm 0 6cm},clip,width=\ImageWidthGT\linewidth]{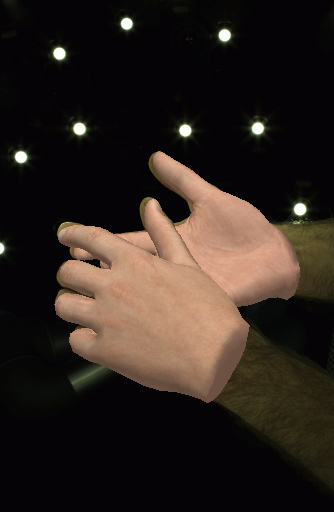}};
  \node[left=\TitleHSepGT of image_GT_1, anchor=south, rotate=90] {\small{Cam View}};
  %
  % second row, left side
  \node[below=\ImageVSepGT of image_GT_1] (image_GT_1_novel) {\includegraphics[trim={0 4cm 0 4cm},clip, width=\ImageWidthGT\linewidth]{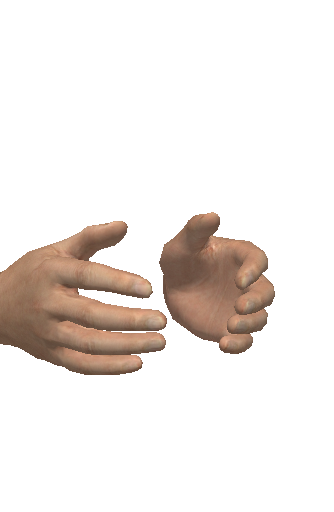}};
  \node[right=\ImageHSepGT of image_GT_1_novel, anchor=west] (image_S_1_1_novel) {\includegraphics[trim={0 4cm 0 4cm},clip,width=\ImageWidthGT\linewidth]{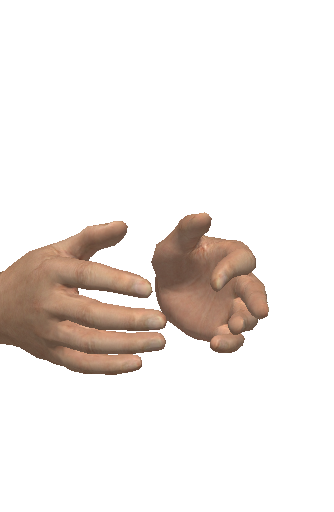}};
  \node[right=\ImageHSepGT of image_S_1_1_novel, anchor=west] (image_S_1_2_novel) {\includegraphics[trim={0 4cm 0 4cm},clip,width=\ImageWidthGT\linewidth]{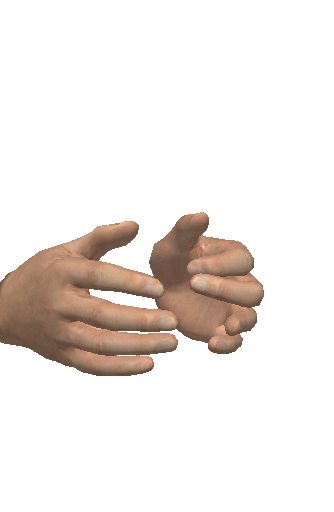}};
  \node[right=\ImageHSepGT of image_S_1_2_novel, anchor=west] (image_S_1_3_novel) {\includegraphics[trim={0 4cm 0 4cm},clip,width=\ImageWidthGT\linewidth]{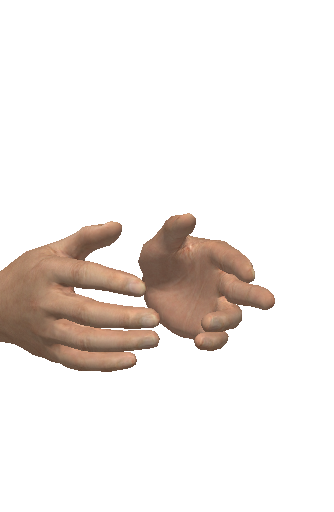}};
  %
  % second row, right side
  \node[right=\ImageBlockHSepGT of image_S_1_3_novel, anchor=west] (image_GT_2_novel) {\includegraphics[trim={0 3cm 0 5cm},clip,width=\ImageWidthGT\linewidth]{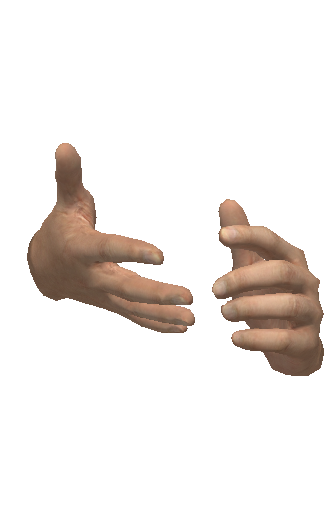}};
  \node[right=\ImageHSepGT of image_GT_2_novel, anchor=west] (image_S_2_1_novel) {\includegraphics[trim={0 3cm 0 5cm},clip,width=\ImageWidthGT\linewidth]{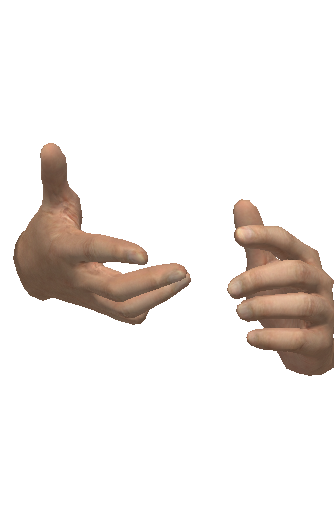}};
  \node[right=\ImageHSepGT of image_S_2_1_novel, anchor=west] (image_S_2_2_novel) {\includegraphics[trim={0 3cm 0 5cm},clip,width=\ImageWidthGT\linewidth]{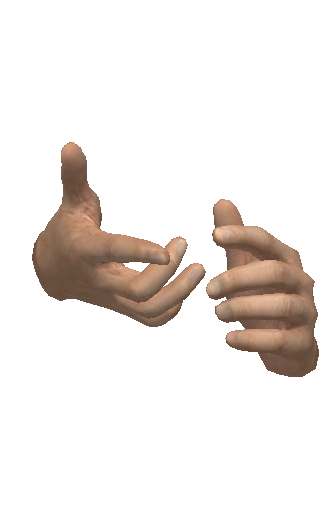}};
  \node[right=\ImageHSepGT of image_S_2_2_novel, anchor=west] (image_S_2_3_novel) {\includegraphics[trim={0 3cm 0 5cm},clip,width=\ImageWidthGT\linewidth]{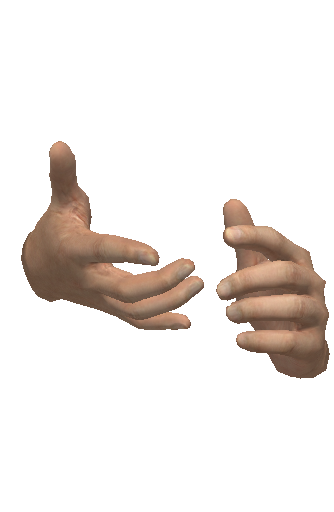}};
  \node[left=\TitleHSepGT of image_GT_1_novel, anchor=south, rotate=90] {\small{Novel View}};
  %
  % third row, left side
  \node[below=\ImageVSepGT of image_GT_1_novel] (image_GT_3) {\includegraphics[trim={0 4cm 0 4cm},clip, width=\ImageWidthGT\linewidth]{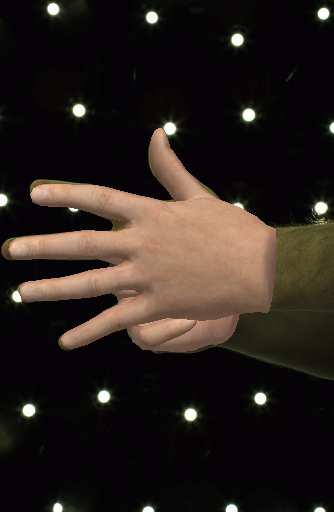}};
  \node[right=\ImageHSepGT of image_GT_3, anchor=west] (image_S_3_1) {\includegraphics[trim={0 4cm 0 4cm},clip, width=\ImageWidthGT\linewidth]{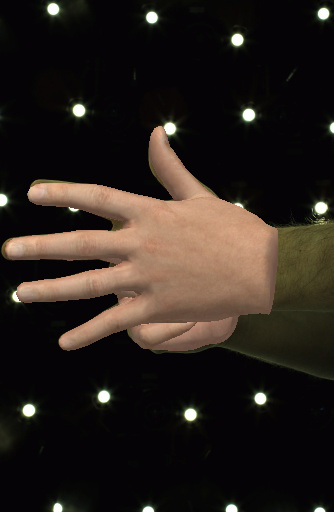}};
  \node[right=\ImageHSepGT of image_S_3_1, anchor=west] (image_S_3_2) {\includegraphics[trim={0 4cm 0 4cm},clip, width=\ImageWidthGT\linewidth]{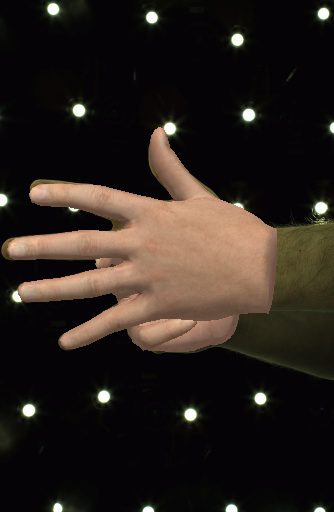}};
  \node[right=\ImageHSepGT of image_S_3_2, anchor=west] (image_S_3_3)
  {\includegraphics[trim={0 4cm 0 4cm},clip, width=\ImageWidthGT\linewidth]{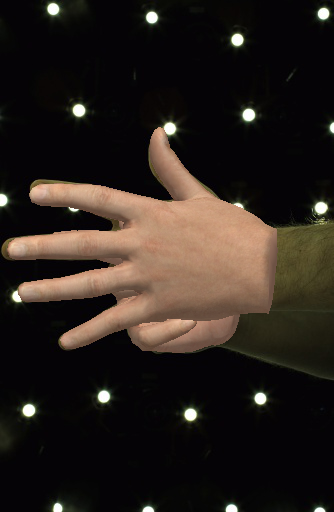}};
  %
  % third row, right side
  \node[right=\ImageBlockHSepGT of image_S_3_3, anchor=west] (image_GT_4) {\includegraphics[trim={0 2cm 0 6cm},clip,width=\ImageWidthGT\linewidth]{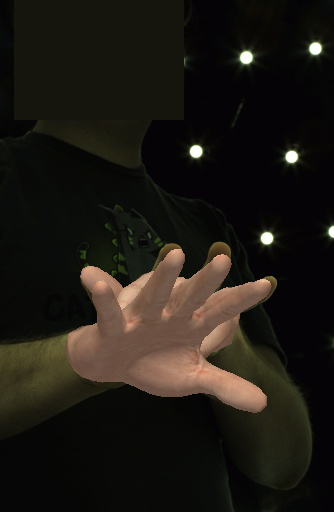}};
  \node[right=\ImageHSepGT of image_GT_4, anchor=west] (image_S_4_1) {\includegraphics[trim={0 2cm 0 6cm},clip,width=\ImageWidthGT\linewidth]{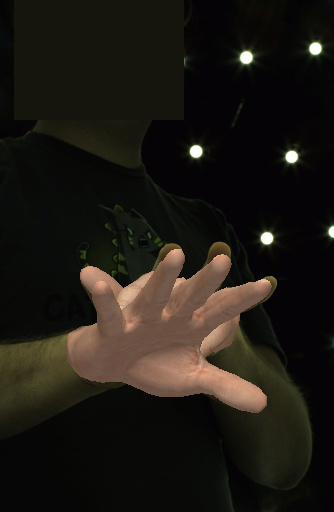}};
  \node[right=\ImageHSepGT of image_S_4_1, anchor=west] (image_S_4_2) {\includegraphics[trim={0 2cm 0 6cm},clip,width=\ImageWidthGT\linewidth]{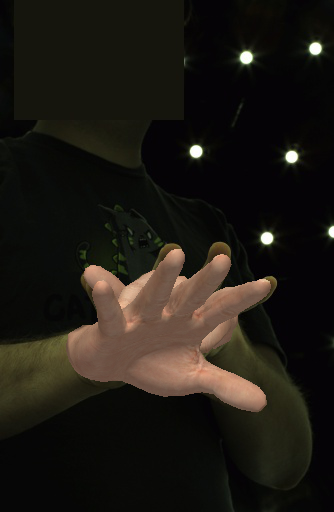}};
  \node[right=\ImageHSepGT of image_S_4_2, anchor=west] (image_S_4_3) {\includegraphics[trim={0 2cm 0 6cm},clip,width=\ImageWidthGT\linewidth]{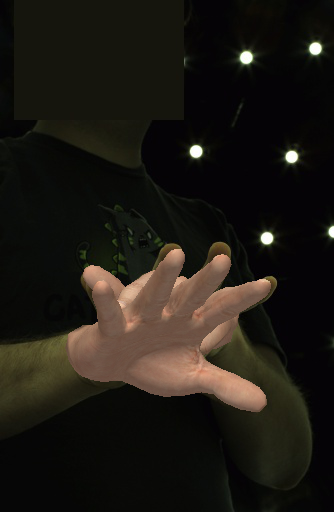}};
  \node[left=\TitleHSepGT of image_GT_3, anchor=south, rotate=90] {\small{Cam View}};
  %
  % fourth row, left side
  \node[below=\ImageVSepGT of image_GT_3] (image_GT_3_novel) {\includegraphics[trim={0 4cm 0 4cm},clip, width=\ImageWidthGT\linewidth]{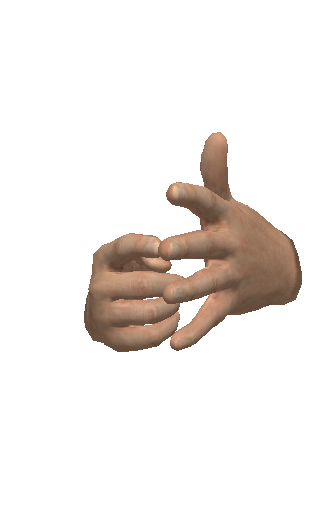}};
  \node[right=\ImageHSepGT of image_GT_3_novel, anchor=west] (image_S_3_1_novel) {\includegraphics[trim={0 4cm 0 4cm},clip,width=\ImageWidthGT\linewidth]{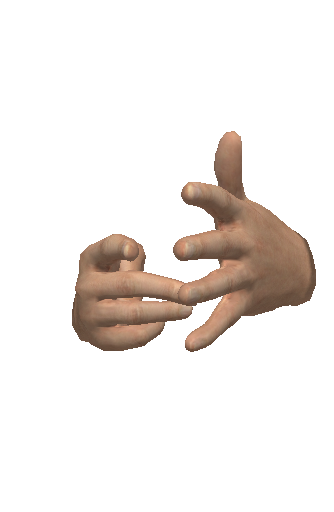}};
  \node[right=\ImageHSepGT of image_S_3_1_novel, anchor=west] (image_S_3_2_novel) {\includegraphics[trim={0 4cm 0 4cm},clip,width=\ImageWidthGT\linewidth]{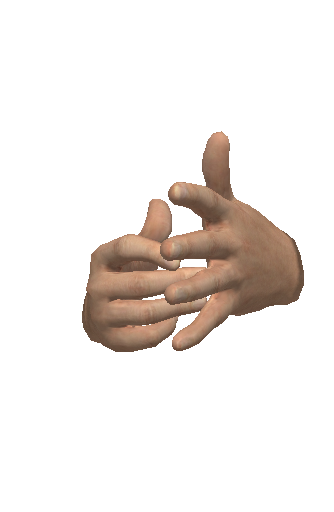}};
  \node[right=\ImageHSepGT of image_S_3_2_novel, anchor=west] (image_S_3_3_novel) {\includegraphics[trim={0 4cm 0 4cm},clip,width=\ImageWidthGT\linewidth]{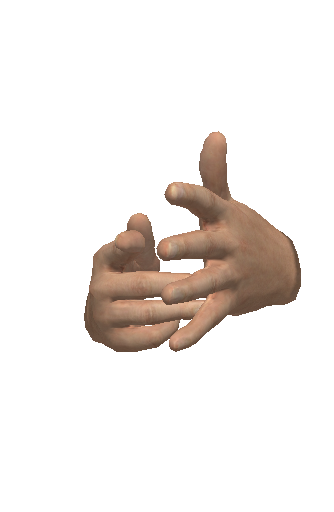}};
  %
  % fourth row, right side
  \node[right=\ImageBlockHSepGT of image_S_3_3_novel, anchor=west] (image_GT_4_novel) {\includegraphics[trim={0 3cm 0 5cm},clip,width=\ImageWidthGT\linewidth]{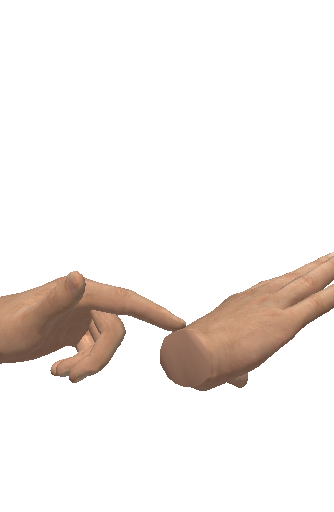}};
  \node[right=\ImageHSepGT of image_GT_4_novel, anchor=west] (image_S_4_1_novel) {\includegraphics[trim={0 3cm 0 5cm},clip,width=\ImageWidthGT\linewidth]{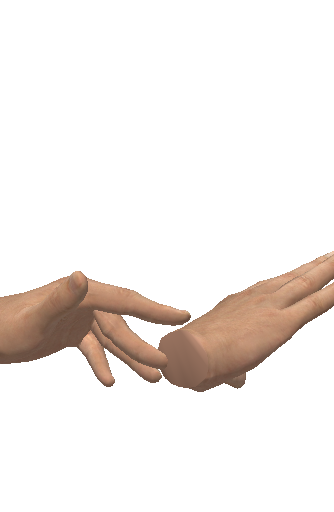}};
  \node[right=\ImageHSepGT of image_S_4_1_novel, anchor=west] (image_S_4_2_novel) {\includegraphics[trim={0 3cm 0 5cm},clip,width=\ImageWidthGT\linewidth]{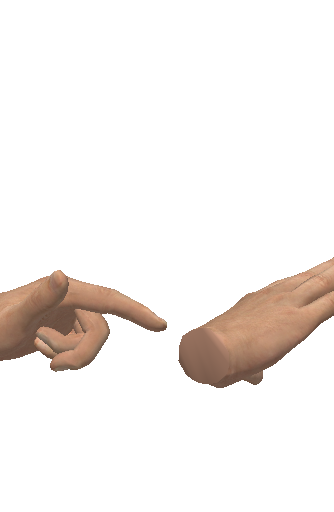}};
  \node[right=\ImageHSepGT of image_S_4_2_novel, anchor=west] (image_S_4_3_novel) {\includegraphics[trim={0 3cm 0 5cm},clip,width=\ImageWidthGT\linewidth]{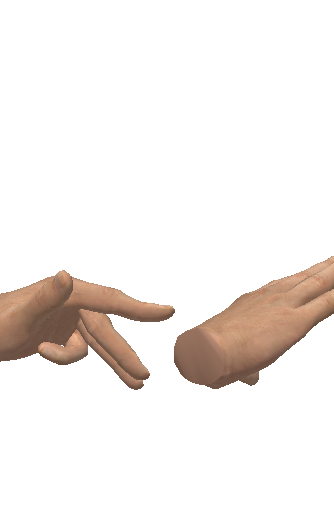}};
  \node[left=\TitleHSepGT of image_GT_3_novel, anchor=south, rotate=90] {\small{Novel View}};
  %
  % fifth row, left side
  \node[below=\ImageVSepGT of image_GT_3_novel] (image_GT_5) {\includegraphics[trim={0 4cm 0 4cm},clip, width=\ImageWidthGT\linewidth]{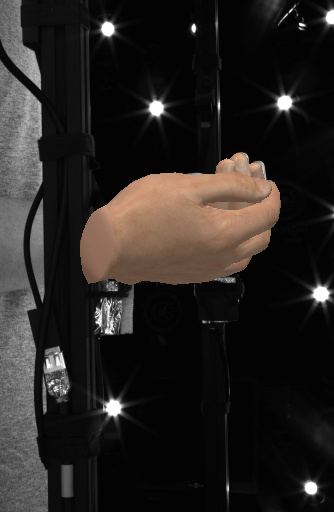}};
  \node[right=\ImageHSepGT of image_GT_5, anchor=west] (image_S_5_1) {\includegraphics[trim={0 4cm 0 4cm},clip, width=\ImageWidthGT\linewidth]{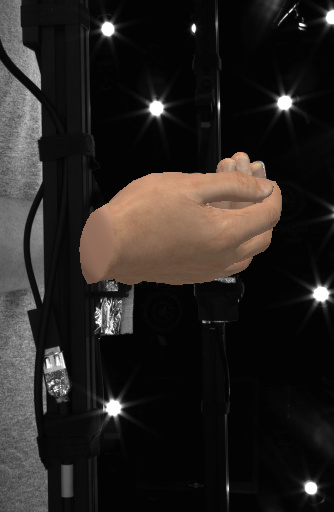}};
  \node[right=\ImageHSepGT of image_S_5_1, anchor=west] (image_S_5_2) {\includegraphics[trim={0 4cm 0 4cm},clip, width=\ImageWidthGT\linewidth]{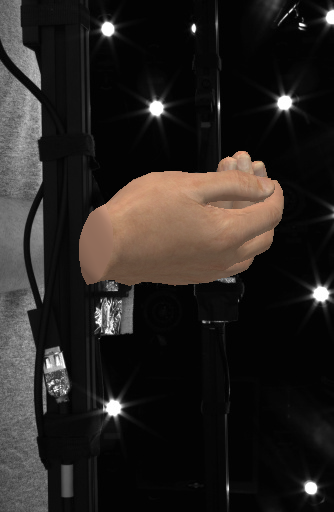}};
  \node[right=\ImageHSepGT of image_S_5_2, anchor=west] (image_S_5_3)
  {\includegraphics[trim={0 4cm 0 4cm},clip, width=\ImageWidthGT\linewidth]{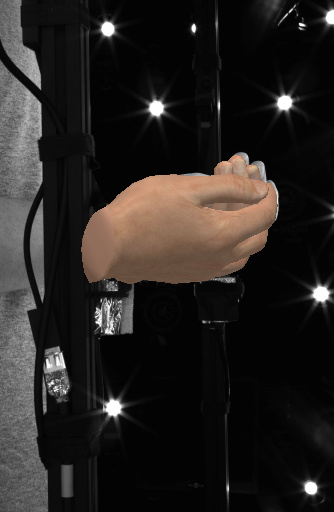}};
  %
  % fifth row, right side
  \node[right=\ImageBlockHSepGT of image_S_5_3, anchor=west] (image_GT_6) {\includegraphics[trim={0 2cm 0 6cm},clip,width=\ImageWidthGT\linewidth]{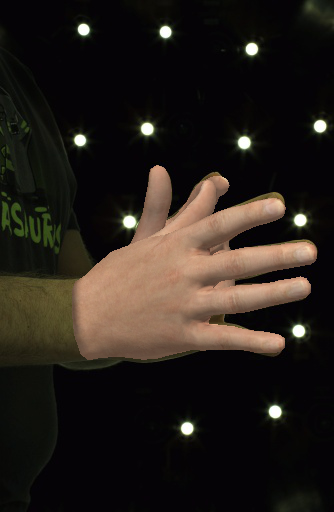}};
  \node[right=\ImageHSepGT of image_GT_6, anchor=west] (image_S_6_1) {\includegraphics[trim={0 2cm 0 6cm},clip,width=\ImageWidthGT\linewidth]{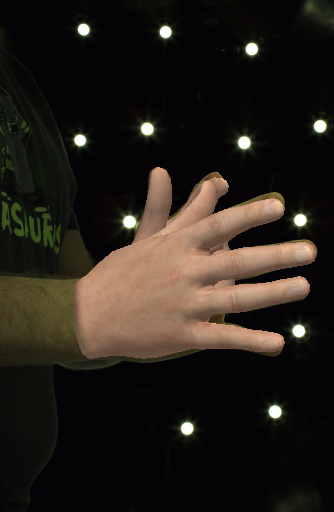}};
  \node[right=\ImageHSepGT of image_S_6_1, anchor=west] (image_S_6_2) {\includegraphics[trim={0 2cm 0 6cm},clip,width=\ImageWidthGT\linewidth]{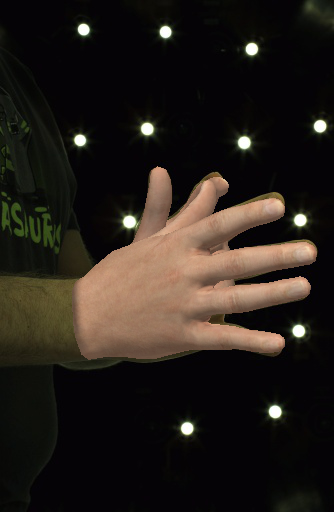}};
  \node[right=\ImageHSepGT of image_S_6_2, anchor=west] (image_S_6_3) {\includegraphics[trim={0 2cm 0 6cm},clip,width=\ImageWidthGT\linewidth]{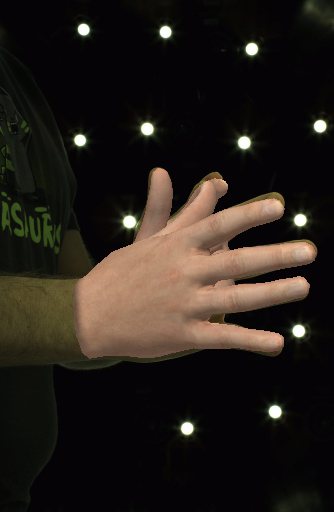}};
  \node[left=\TitleHSepGT of image_GT_5, anchor=south, rotate=90] {\small{Cam View}};
  %
  % sixth row, left side
  \node[below=\ImageVSepGT of image_GT_5] (image_GT_5_novel) {\includegraphics[trim={0 4cm 0 4cm},clip, width=\ImageWidthGT\linewidth]{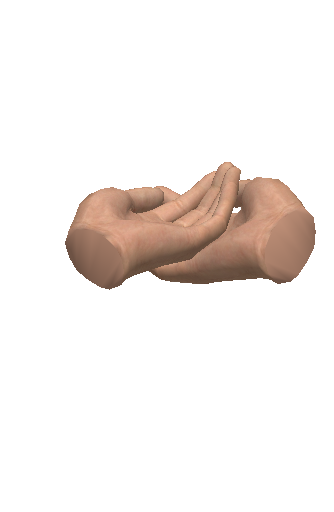}};
  \node[right=\ImageHSepGT of image_GT_5_novel, anchor=west] (image_S_5_1_novel) {\includegraphics[trim={0 4cm 0 4cm},clip,width=\ImageWidthGT\linewidth]{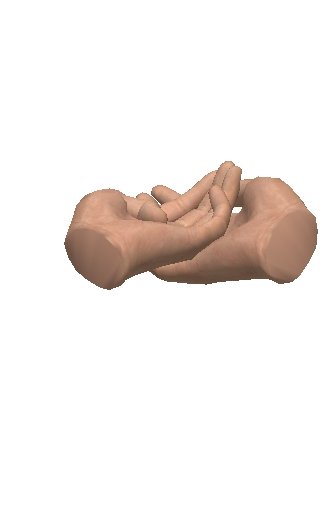}};
  \node[right=\ImageHSepGT of image_S_5_1_novel, anchor=west] (image_S_5_2_novel) {\includegraphics[trim={0 4cm 0 4cm},clip,width=\ImageWidthGT\linewidth]{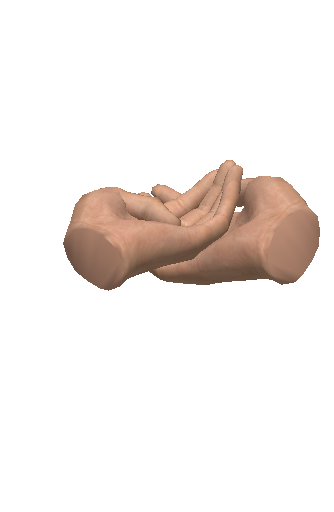}};
  \node[right=\ImageHSepGT of image_S_5_2_novel, anchor=west] (image_S_5_3_novel) {\includegraphics[trim={0 4cm 0 4cm},clip,width=\ImageWidthGT\linewidth]{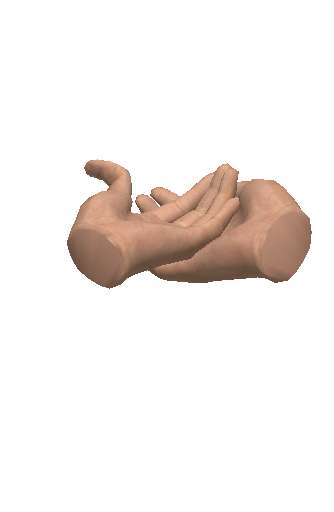}};
  %
  % sixth row, right side
  \node[right=\ImageBlockHSepGT of image_S_5_3_novel, anchor=west] (image_GT_6_novel) {\includegraphics[trim={0 3cm 0 5cm},clip,width=\ImageWidthGT\linewidth]{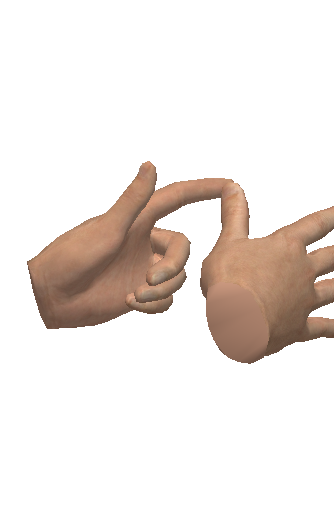}};
  \node[right=\ImageHSepGT of image_GT_6_novel, anchor=west] (image_S_6_1_novel) {\includegraphics[trim={0 3cm 0 5cm},clip,width=\ImageWidthGT\linewidth]{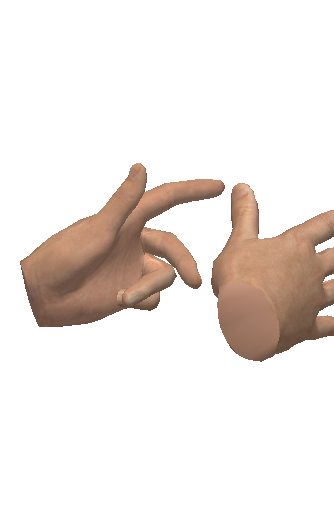}};
  \node[right=\ImageHSepGT of image_S_6_1_novel, anchor=west] (image_S_6_2_novel) {\includegraphics[trim={0 3cm 0 5cm},clip,width=\ImageWidthGT\linewidth]{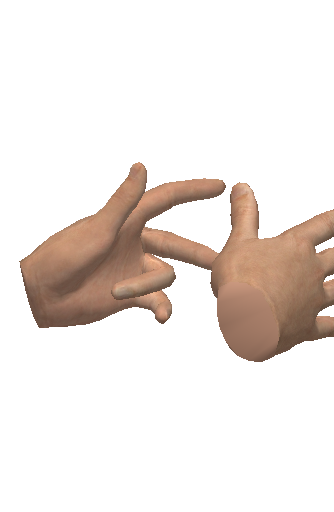}};
  \node[right=\ImageHSepGT of image_S_6_2_novel, anchor=west] (image_S_6_3_novel) {\includegraphics[trim={0 3cm 0 5cm},clip,width=\ImageWidthGT\linewidth]{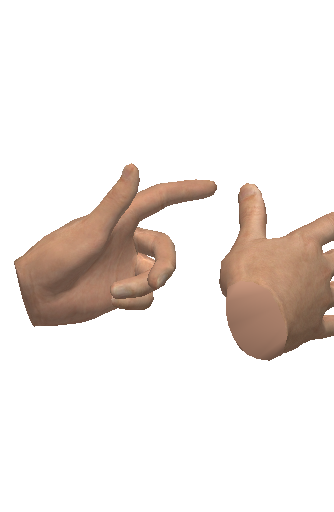}};
  \node[left=\TitleHSepGT of image_GT_5_novel, anchor=south, rotate=90] {\small{Novel View}};

  \foreach \i in {1,...,6}
  {
  \node[draw,\BoxThicknessGT,fit=(image_GT_\i_novel)] {};
  \node[draw,\BoxThicknessGT,fit=(image_S_\i_3_novel)] {};
  \node[draw,\BoxThicknessGT,fit=(image_S_\i_1_novel)] {};
  \node[draw,\BoxThicknessGT,fit=(image_S_\i_1_novel) (image_S_\i_2_novel) (image_S_\i_3_novel)] {};
  
  \node[draw,\BoxThicknessGT,fit=(image_GT_\i)] {};
  \node[draw,\BoxThicknessGT,fit=(image_S_\i_3)] {};
  \node[draw,\BoxThicknessGT,fit=(image_S_\i_1)] {};
  \node[draw,\BoxThicknessGT,fit=(image_S_\i_1) (image_S_\i_2) (image_S_\i_3)] {};
  }
  \end{tikzpicture}

  \caption{More visualizations of the our MultiHands dataset. Note the diversity of 3D poses that can be seen in the novel view. 
  }
  \label{fig:gt_vis_sup}
\end{figure*}
