# Supplementary material for: HandFlow: Quantifying View-Dependent 3D Ambiguity in Two-Hand Reconstruction with Normalizing Flow
Source: arXiv:2210.01692 source file (2022-10-04)
Supplement: Supplementary file 4 [file OverlayResults_new.tex]

{
\newcommand{\ImageWidthSupp}{0.118}
\newcommand{\ImageHSepSupp}{0.05cm}
\newcommand{\ImageVSepSupp}{0.05cm}
\newcommand{\ImageBlockHSepSupp}{0.2cm}
\newcommand{\ImageBlockVSepSupp}{0.2cm}
\newcommand{\TitleHSepSupp}{0.15cm}
\newcommand{\TitleVSepSupp}{0.35cm}
\newcommand{\BoxThicknessSupp}{semithick}
\begin{figure*}
  \centering
  \begin{tikzpicture}[every node/.style={inner sep=0,outer sep=0}]%
  % first row, left side
  \node (image_GT_1) at (0,0) {\includegraphics[width=\ImageWidthSupp\linewidth]{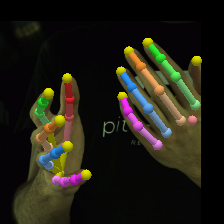}};
  \node[above=\TitleVSepSupp of image_GT_1, anchor=north] {\small{Ground Truth}};
  \node[right=\ImageHSepSupp of image_GT_1, anchor=west] (image_S_1_1) {\includegraphics[width=\ImageWidthSupp\linewidth]{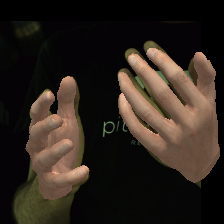}};
  \node[right=\ImageHSepSupp of image_S_1_1, anchor=west] (image_S_1_2) {\includegraphics[width=\ImageWidthSupp\linewidth]{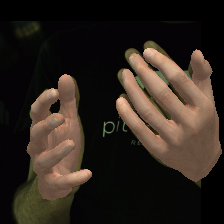}};
  \node[above=\TitleVSepSupp of image_S_1_2, anchor=north] {\small{Our Samples}};
  \node[right=\ImageHSepSupp of image_S_1_2, anchor=west] (image_S_1_3) {\includegraphics[width=\ImageWidthSupp\linewidth]{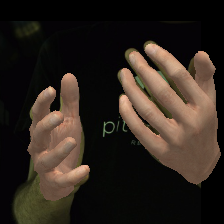}};
  %
  % first row, right side
  \node[right=\ImageBlockHSepSupp of image_S_1_3, anchor=west] (image_GT_2) {\includegraphics[width=\ImageWidthSupp\linewidth]{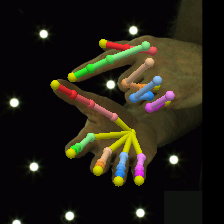}};
  \node[above=\TitleVSepSupp of image_GT_2, anchor=north] {\small{Ground Truth}};
  \node[right=\ImageHSepSupp of image_GT_2, anchor=west] (image_S_2_1) {\includegraphics[width=\ImageWidthSupp\linewidth]{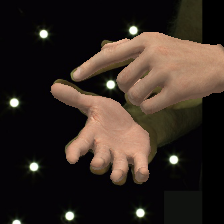}};
  \node[right=\ImageHSepSupp of image_S_2_1, anchor=west] (image_S_2_2) {\includegraphics[width=\ImageWidthSupp\linewidth]{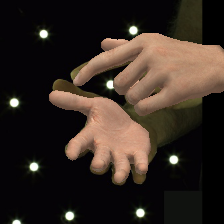}};
  \node[above=\TitleVSepSupp of image_S_2_2, anchor=north] {\small{Our Samples}};
  \node[right=\ImageHSepSupp of image_S_2_2, anchor=west] (image_S_2_3) {\includegraphics[width=\ImageWidthSupp\linewidth]{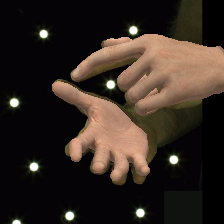}};
  \node[left=\TitleHSepSupp of image_GT_1, anchor=south, rotate=90] {\small{Cam View}};
  %
  % second row, left side
  \node[below=\ImageVSepSupp of image_GT_1] (image_GT_1_novel) {\includegraphics[trim={0 0cm 0 1cm},clip, width=\ImageWidthSupp\linewidth]{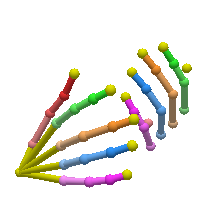}};
  \node[right=\ImageHSepSupp of image_GT_1_novel, anchor=west] (image_S_1_1_novel) {\includegraphics[trim={0 0cm 0 1cm},clip,width=\ImageWidthSupp\linewidth]{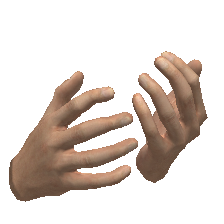}};
  \node[right=\ImageHSepSupp of image_S_1_1_novel, anchor=west] (image_S_1_2_novel) {\includegraphics[trim={0 0cm 0 1cm},clip,width=\ImageWidthSupp\linewidth]{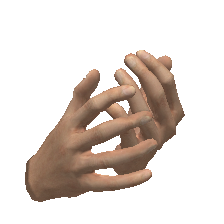}};
  \node[right=\ImageHSepSupp of image_S_1_2_novel, anchor=west] (image_S_1_3_novel) {\includegraphics[trim={0 0cm 0 1cm},clip,width=\ImageWidthSupp\linewidth]{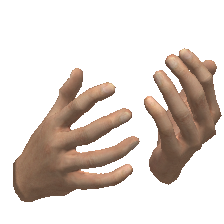}};
  %
  % second row, right side
  \node[right=\ImageBlockHSepSupp of image_S_1_3_novel, anchor=west] (image_GT_2_novel) {\includegraphics[trim={0 0cm 0 1cm},clip,width=\ImageWidthSupp\linewidth]{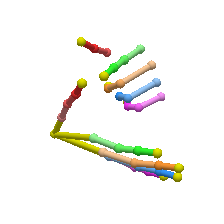}};
  \node[right=\ImageHSepSupp of image_GT_2_novel, anchor=west] (image_S_2_1_novel) {\includegraphics[trim={0 0cm 0 1cm},clip,width=\ImageWidthSupp\linewidth]{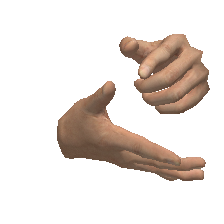}};
  \node[right=\ImageHSepSupp of image_S_2_1_novel, anchor=west] (image_S_2_2_novel) {\includegraphics[trim={0 0cm 0 1cm},clip,width=\ImageWidthSupp\linewidth]{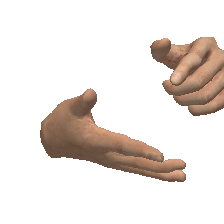}};
  \node[right=\ImageHSepSupp of image_S_2_2_novel, anchor=west] (image_S_2_3_novel) {\includegraphics[trim={0 0cm 0 1cm},clip,width=\ImageWidthSupp\linewidth]{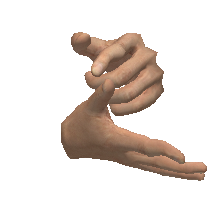}};
  \node[left=\TitleHSepSupp of image_GT_1_novel, anchor=south, rotate=90] {\small{Novel View}};
  %
  % third row, left side
  \node[below=\ImageBlockVSepSupp of image_GT_1_novel] (image_GT_3) {\includegraphics[width=\ImageWidthSupp\linewidth]{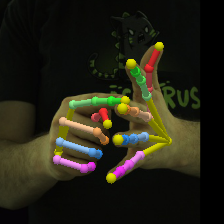}};
  \node[right=\ImageHSepSupp of image_GT_3, anchor=west] (image_S_3_1) {\includegraphics[width=\ImageWidthSupp\linewidth]{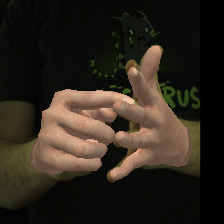}};
  \node[right=\ImageHSepSupp of image_S_3_1, anchor=west] (image_S_3_2) {\includegraphics[width=\ImageWidthSupp\linewidth]{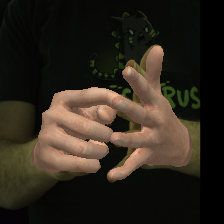}};
  \node[right=\ImageHSepSupp of image_S_3_2, anchor=west] (image_S_3_3) {\includegraphics[width=\ImageWidthSupp\linewidth]{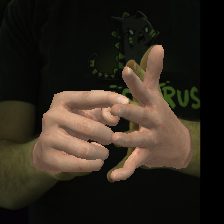}};
  %
  % third row, right side
  \node[right=\ImageBlockHSepSupp of image_S_3_3, anchor=west] (image_GT_4) {\includegraphics[width=\ImageWidthSupp\linewidth]{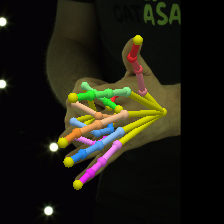}};
  \node[right=\ImageHSepSupp of image_GT_4, anchor=west] (image_S_4_1) {\includegraphics[width=\ImageWidthSupp\linewidth]{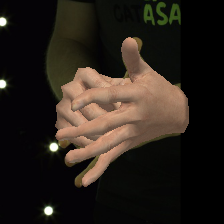}};
  \node[right=\ImageHSepSupp of image_S_4_1, anchor=west] (image_S_4_2) {\includegraphics[width=\ImageWidthSupp\linewidth]{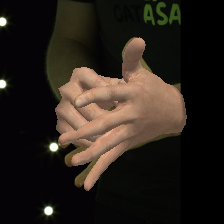}};
  \node[right=\ImageHSepSupp of image_S_4_2, anchor=west] (image_S_4_3) {\includegraphics[width=\ImageWidthSupp\linewidth]{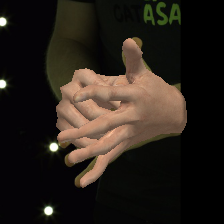}};
  \node[left=\TitleHSepSupp of image_GT_3, anchor=south, rotate=90] {\small{Cam View}};
  %
  % fourth row, left side
  \node[below=\ImageVSepSupp of image_GT_3] (image_GT_3_novel) {\includegraphics[width=\ImageWidthSupp\linewidth]{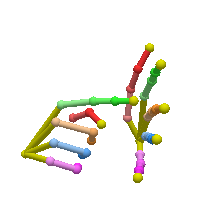}};
  \node[right=\ImageHSepSupp of image_GT_3_novel, anchor=west] (image_S_3_1_novel) {\includegraphics[width=\ImageWidthSupp\linewidth]{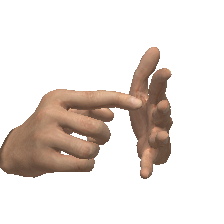}};
  \node[right=\ImageHSepSupp of image_S_3_1_novel, anchor=west] (image_S_3_2_novel) {\includegraphics[width=\ImageWidthSupp\linewidth]{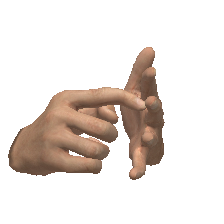}};
  \node[right=\ImageHSepSupp of image_S_3_2_novel, anchor=west] (image_S_3_3_novel) {\includegraphics[width=\ImageWidthSupp\linewidth]{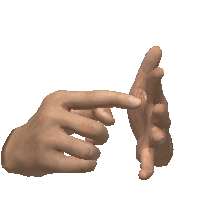}};
  %
  % fourth row, right side
  \node[right=\ImageBlockHSepSupp of image_S_3_3_novel, anchor=west] (image_GT_4_novel) {\includegraphics[width=\ImageWidthSupp\linewidth]{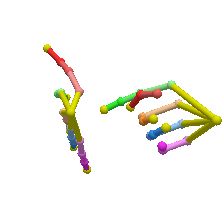}};
  \node[right=\ImageHSepSupp of image_GT_4_novel, anchor=west] (image_S_4_1_novel) {\includegraphics[width=\ImageWidthSupp\linewidth]{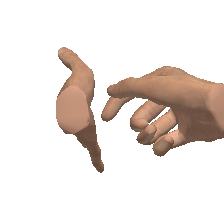}};
  \node[right=\ImageHSepSupp of image_S_4_1_novel, anchor=west] (image_S_4_2_novel) {\includegraphics[width=\ImageWidthSupp\linewidth]{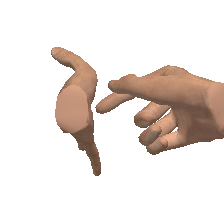}};
  \node[right=\ImageHSepSupp of image_S_4_2_novel, anchor=west] (image_S_4_3_novel) {\includegraphics[width=\ImageWidthSupp\linewidth]{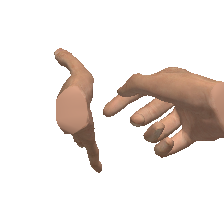}};
  \node[left=\TitleHSepSupp of image_GT_3_novel, anchor=south, rotate=90] {\small{Novel View}};
  %
  % fifth row, left side
  \node[below=\ImageBlockVSepSupp of image_GT_3_novel] (image_GT_5) {\includegraphics[width=\ImageWidthSupp\linewidth]{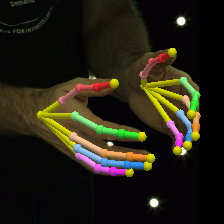}};
  \node[right=\ImageHSepSupp of image_GT_5, anchor=west] (image_S_5_1) {\includegraphics[width=\ImageWidthSupp\linewidth]{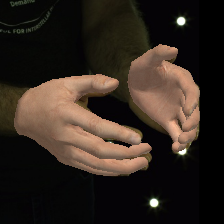}};
  \node[right=\ImageHSepSupp of image_S_5_1, anchor=west] (image_S_5_2) {\includegraphics[width=\ImageWidthSupp\linewidth]{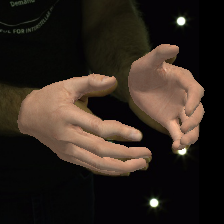}};
  \node[right=\ImageHSepSupp of image_S_5_2, anchor=west] (image_S_5_3) {\includegraphics[width=\ImageWidthSupp\linewidth]{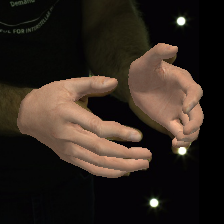}};
  %
  % fifth row, right side
  \node[right=\ImageBlockHSepSupp of image_S_5_3, anchor=west] (image_GT_6) {\includegraphics[width=\ImageWidthSupp\linewidth]{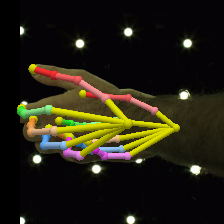}};
  \node[right=\ImageHSepSupp of image_GT_6, anchor=west] (image_S_6_1) {\includegraphics[width=\ImageWidthSupp\linewidth]{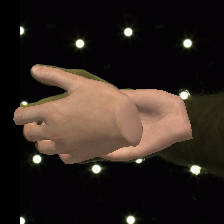}};
  \node[right=\ImageHSepSupp of image_S_6_1, anchor=west] (image_S_6_2) {\includegraphics[width=\ImageWidthSupp\linewidth]{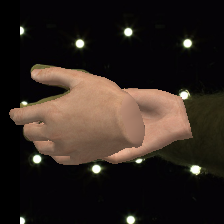}};
  \node[right=\ImageHSepSupp of image_S_6_2, anchor=west] (image_S_6_3) {\includegraphics[width=\ImageWidthSupp\linewidth]{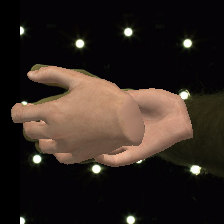}};
  \node[left=\TitleHSepSupp of image_GT_5, anchor=south, rotate=90] {\small{Cam View}};
  %
  % sixth row, left side
  \node[below=\ImageVSepSupp of image_GT_5] (image_GT_5_novel) {\includegraphics[width=\ImageWidthSupp\linewidth]{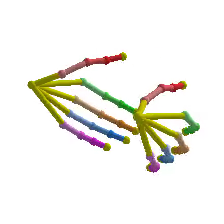}};
  \node[right=\ImageHSepSupp of image_GT_5_novel, anchor=west] (image_S_5_1_novel) {\includegraphics[width=\ImageWidthSupp\linewidth]{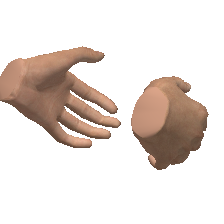}};
  \node[right=\ImageHSepSupp of image_S_5_1_novel, anchor=west] (image_S_5_2_novel) {\includegraphics[width=\ImageWidthSupp\linewidth]{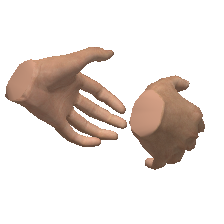}};
  \node[right=\ImageHSepSupp of image_S_5_2_novel, anchor=west] (image_S_5_3_novel) {\includegraphics[width=\ImageWidthSupp\linewidth]{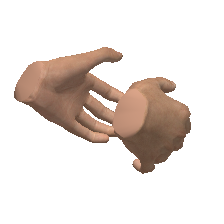}};
  %
  % sixth row, right side
  \node[right=\ImageBlockHSepSupp of image_S_5_3_novel, anchor=west] (image_GT_6_novel) {\includegraphics[width=\ImageWidthSupp\linewidth]{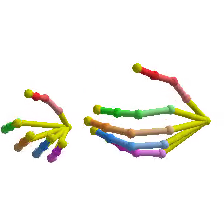}};
  \node[right=\ImageHSepSupp of image_GT_6_novel, anchor=west] (image_S_6_1_novel) {\includegraphics[width=\ImageWidthSupp\linewidth]{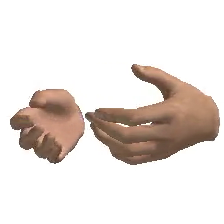}};
  \node[right=\ImageHSepSupp of image_S_6_1_novel, anchor=west] (image_S_6_2_novel) {\includegraphics[width=\ImageWidthSupp\linewidth]{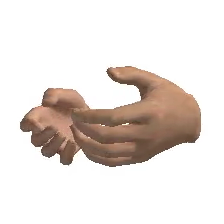}};
  \node[right=\ImageHSepSupp of image_S_6_2_novel, anchor=west] (image_S_6_3_novel) {\includegraphics[width=\ImageWidthSupp\linewidth]{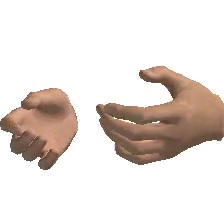}};
  \node[left=\TitleHSepSupp of image_GT_5_novel, anchor=south, rotate=90] {\small{Novel View}};
  %
  % seventh row, left side
  \node[below=\ImageBlockVSepSupp of image_GT_5_novel] (image_GT_7)
  {\includegraphics[width=\ImageWidthSupp\linewidth]{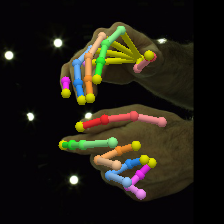}};
  \node[right=\ImageHSepSupp of image_GT_7, anchor=west] (image_S_7_1)
  {\includegraphics[width=\ImageWidthSupp\linewidth]{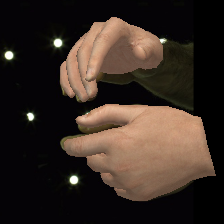}};
  \node[right=\ImageHSepSupp of image_S_7_1, anchor=west] (image_S_7_2)
  {\includegraphics[width=\ImageWidthSupp\linewidth]{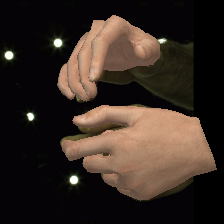}};
  \node[right=\ImageHSepSupp of image_S_7_2, anchor=west] (image_S_7_3)
  {\includegraphics[width=\ImageWidthSupp\linewidth]{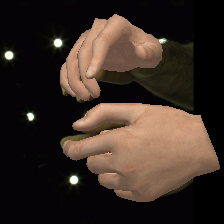}};
  %
  % seventh row, right side
  \node[right=\ImageBlockHSepSupp of image_S_7_3, anchor=west] (image_GT_8)
  {\includegraphics[width=\ImageWidthSupp\linewidth]{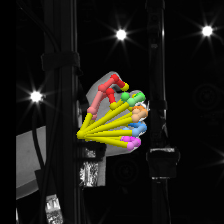}};
  \node[right=\ImageHSepSupp of image_GT_8, anchor=west] (image_S_8_1)
  {\includegraphics[width=\ImageWidthSupp\linewidth]{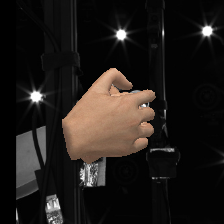}};
  \node[right=\ImageHSepSupp of image_S_8_1, anchor=west] (image_S_8_2)
  {\includegraphics[width=\ImageWidthSupp\linewidth]{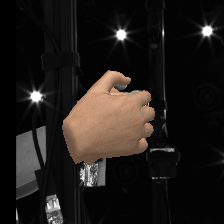}};
  \node[right=\ImageHSepSupp of image_S_8_2, anchor=west] (image_S_8_3)
  {\includegraphics[width=\ImageWidthSupp\linewidth]{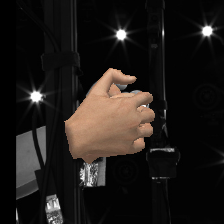}};
  \node[left=\TitleHSepSupp of image_GT_7, anchor=south, rotate=90] {\small{Cam View}};
  %
  % eight row, left side
  \node[below=\ImageVSepSupp of image_GT_7] (image_GT_7_novel) {\includegraphics[width=\ImageWidthSupp\linewidth]{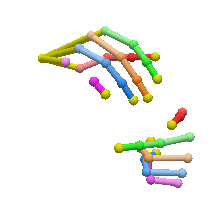}};
  \node[right=\ImageHSepSupp of image_GT_7_novel, anchor=west] (image_S_7_1_novel) {\includegraphics[width=\ImageWidthSupp\linewidth]{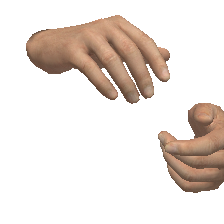}};
  \node[right=\ImageHSepSupp of image_S_7_1_novel, anchor=west] (image_S_7_2_novel) {\includegraphics[width=\ImageWidthSupp\linewidth]{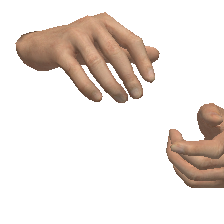}};
  \node[right=\ImageHSepSupp of image_S_7_2_novel, anchor=west] (image_S_7_3_novel) {\includegraphics[width=\ImageWidthSupp\linewidth]{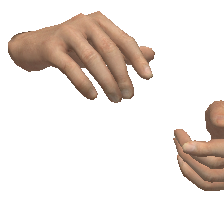}};
  %
  % eight row, right side
  \node[right=\ImageBlockHSepSupp of image_S_7_3_novel, anchor=west] (image_GT_8_novel) {\includegraphics[width=\ImageWidthSupp\linewidth]{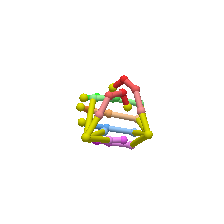}};
  \node[right=\ImageHSepSupp of image_GT_8_novel, anchor=west] (image_S_8_1_novel) {\includegraphics[width=\ImageWidthSupp\linewidth]{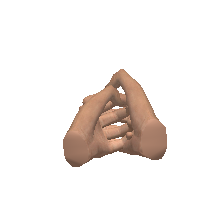}};
  \node[right=\ImageHSepSupp of image_S_8_1_novel, anchor=west] (image_S_8_2_novel) {\includegraphics[width=\ImageWidthSupp\linewidth]{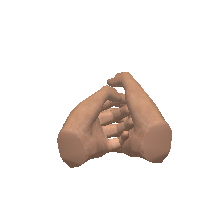}};
  \node[right=\ImageHSepSupp of image_S_8_2_novel, anchor=west] (image_S_8_3_novel) {\includegraphics[width=\ImageWidthSupp\linewidth]{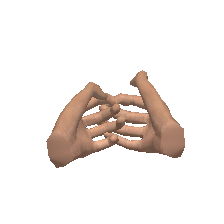}};
  \node[left=\TitleHSepSupp of image_GT_7_novel, anchor=south, rotate=90] {\small{Novel View}};
  \vspace{-0.3cm}
  % boxes
  \foreach \i in {1,...,8}
  {
  \node[draw,\BoxThicknessSupp,fit=(image_GT_\i_novel)] {};
  \node[draw,dash dot dot,\BoxThicknessSupp,fit=(image_S_\i_2_novel)] {};
  \node[draw,\BoxThicknessSupp,fit=(image_S_\i_1_novel) (image_S_\i_2_novel) (image_S_\i_3_novel)] {};
  }
  \end{tikzpicture}
  
  \caption{We show more individual mesh samples from the camera view and from a novel view. Note that not all joints are annotated in the ground truth. This shows up as missing segments in the skeleton.}
  \label{figure:OverlaySupp}
\end{figure*}
}
